# Supplementary material for: DataEvolver: Let Your Data Build and Improve Itself via Goal-Driven Loop Agents
Source: arXiv:2605.01789 source file (2026-05-03)
Supplement: Supplementary file 1 [file v4_external_comparison_supplement.tex]

\section{Supplement: V4 External Comparison Audit}
\label{app:v4-external-comparison}

This supplement collects the denoised V4 audit figures for the reader-facing external comparison: \textbf{Base}, \textbf{Public LoRA}, and \textbf{Ours}. These figures support the main-text claim that the final scene-aware data-construction and feedback-trained model is stronger not only on aggregate metrics but also across angle-level breakdowns.

\subsection{\spatialedit{} Audit Figures}

\begin{figure}[!tbp]
\centering
\includegraphics[width=0.82\linewidth]{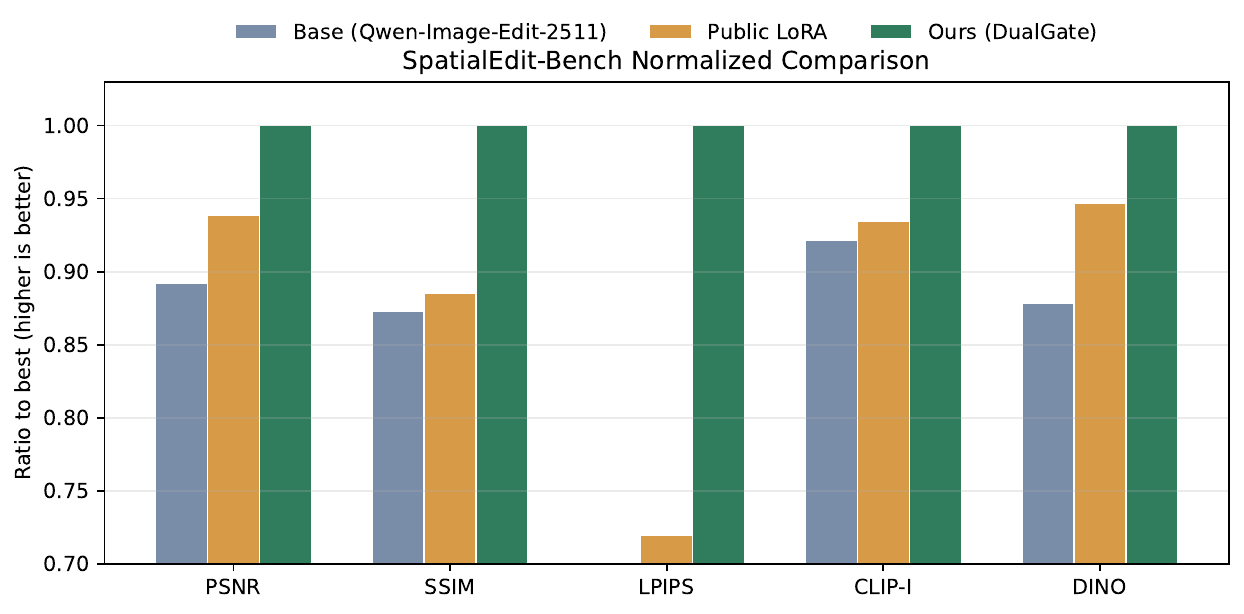}
\caption{Direction-normalized V4 comparison on \spatialedit{}. Positive values indicate improvement after accounting for whether a metric is higher-is-better or lower-is-better.}
\label{fig:v4-spatialedit-normalized}
\end{figure}

\begin{figure}[!tbp]
\centering
\includegraphics[width=0.82\linewidth]{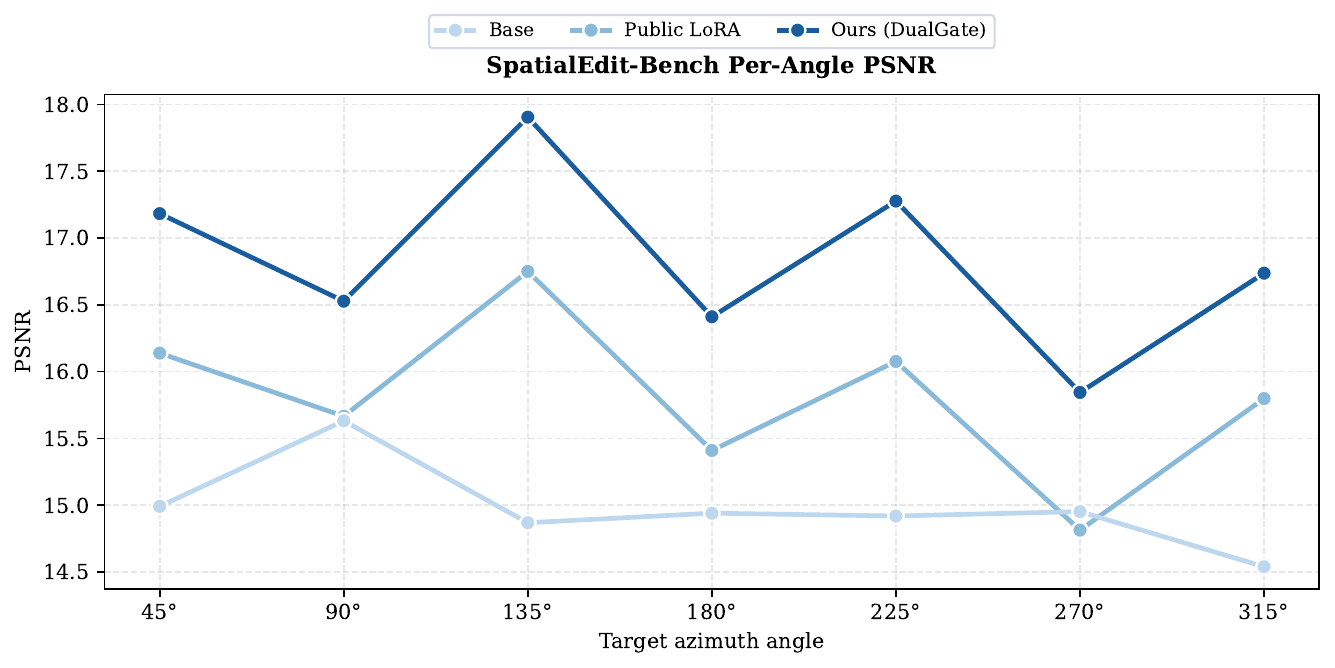}
\caption{Per-angle PSNR audit for the V4 \spatialedit{} comparison. Ours remains strong across the full angle breakdown.}
\label{fig:v4-spatialedit-per-angle-psnr}
\end{figure}

\begin{figure}[!tbp]
\centering
\includegraphics[width=0.82\linewidth]{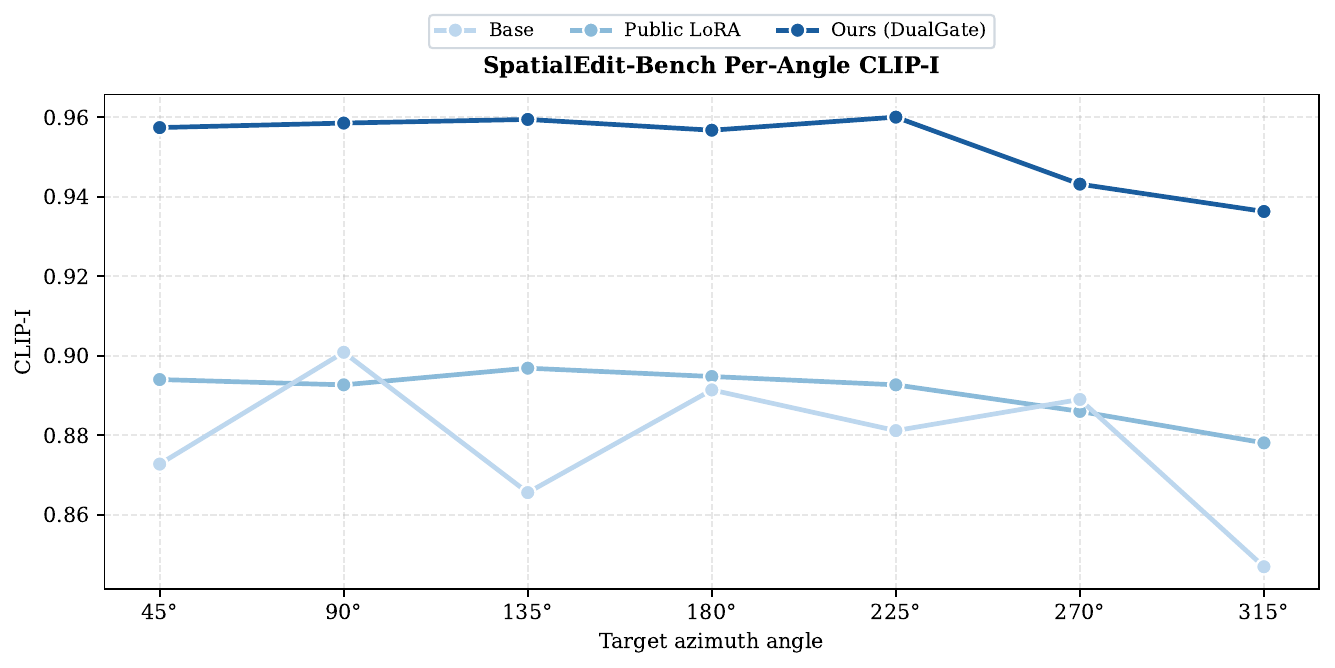}
\caption{Per-angle CLIP-I audit for the V4 \spatialedit{} comparison. Semantic image similarity is consistently stronger for Ours.}
\label{fig:v4-spatialedit-per-angle-clipi}
\end{figure}

\begin{figure}[!tbp]
\centering
\includegraphics[width=0.82\linewidth]{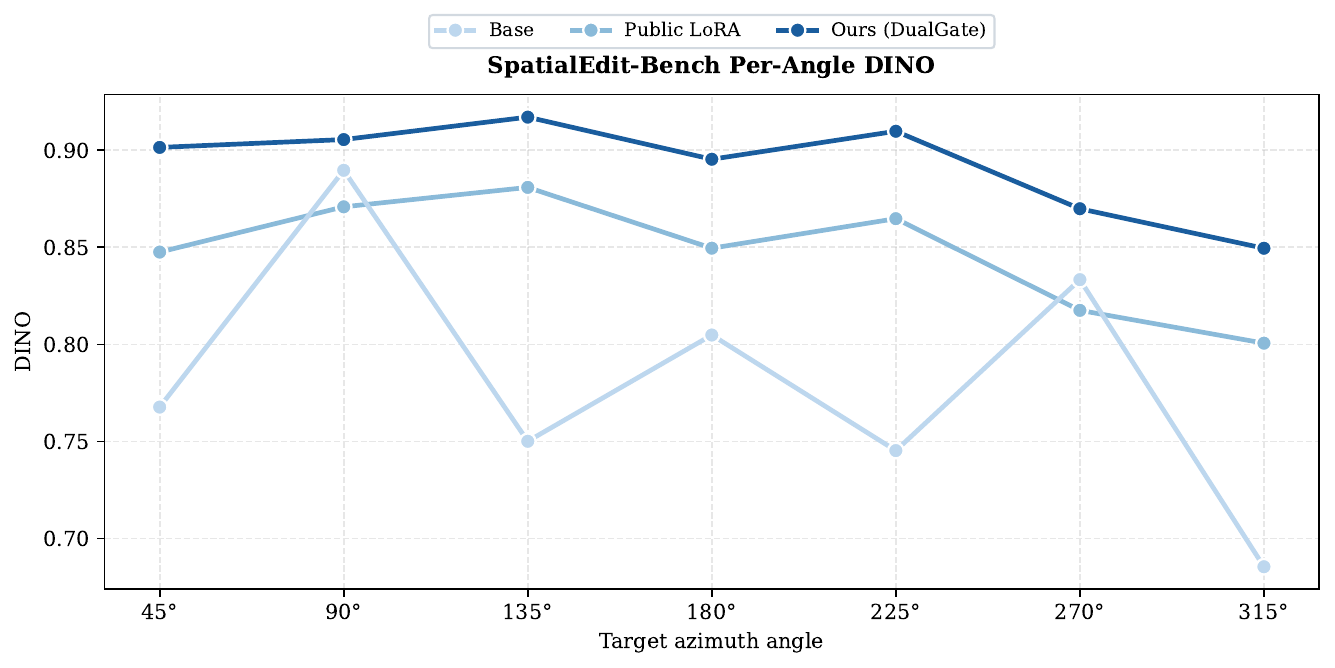}
\caption{Per-angle DINO audit for the V4 \spatialedit{} comparison. Ours maintains stronger identity-sensitive consistency across angles.}
\label{fig:v4-spatialedit-per-angle-dino}
\end{figure}

\subsection{Eval1 Test Set Audit Figures}

\begin{figure}[!tbp]
\centering
\includegraphics[width=0.82\linewidth]{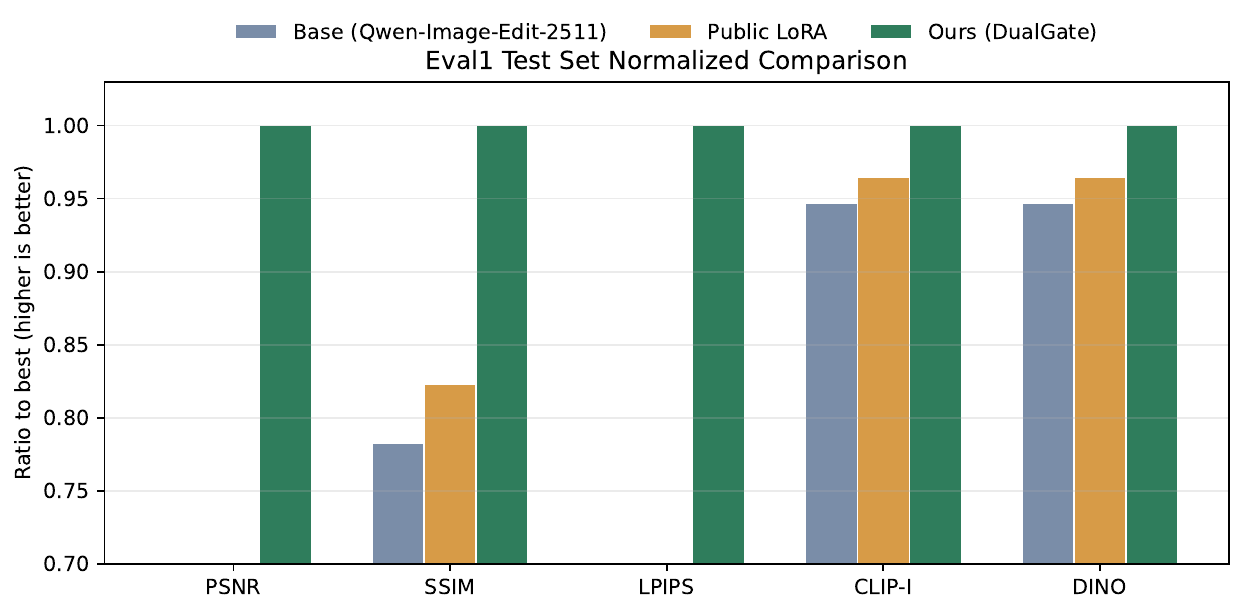}
\caption{Direction-normalized V4 comparison on the Eval1 Test Set. The same reader-facing model ordering is preserved.}
\label{fig:v4-testset-normalized}
\end{figure}

\begin{figure}[!tbp]
\centering
\includegraphics[width=0.82\linewidth]{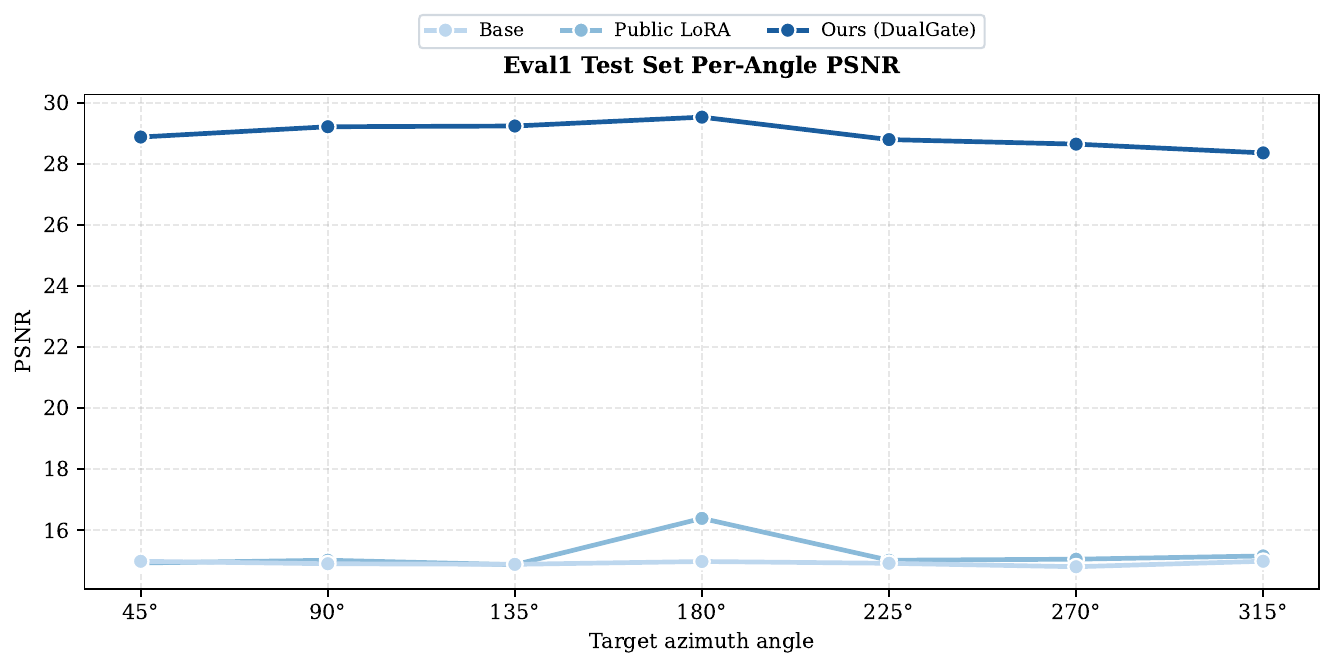}
\caption{Per-angle PSNR audit for the Eval1 Test Set. Ours remains the strongest model across the angle breakdown.}
\label{fig:v4-testset-per-angle-psnr}
\end{figure}

\begin{figure}[!tbp]
\centering
\includegraphics[width=0.82\linewidth]{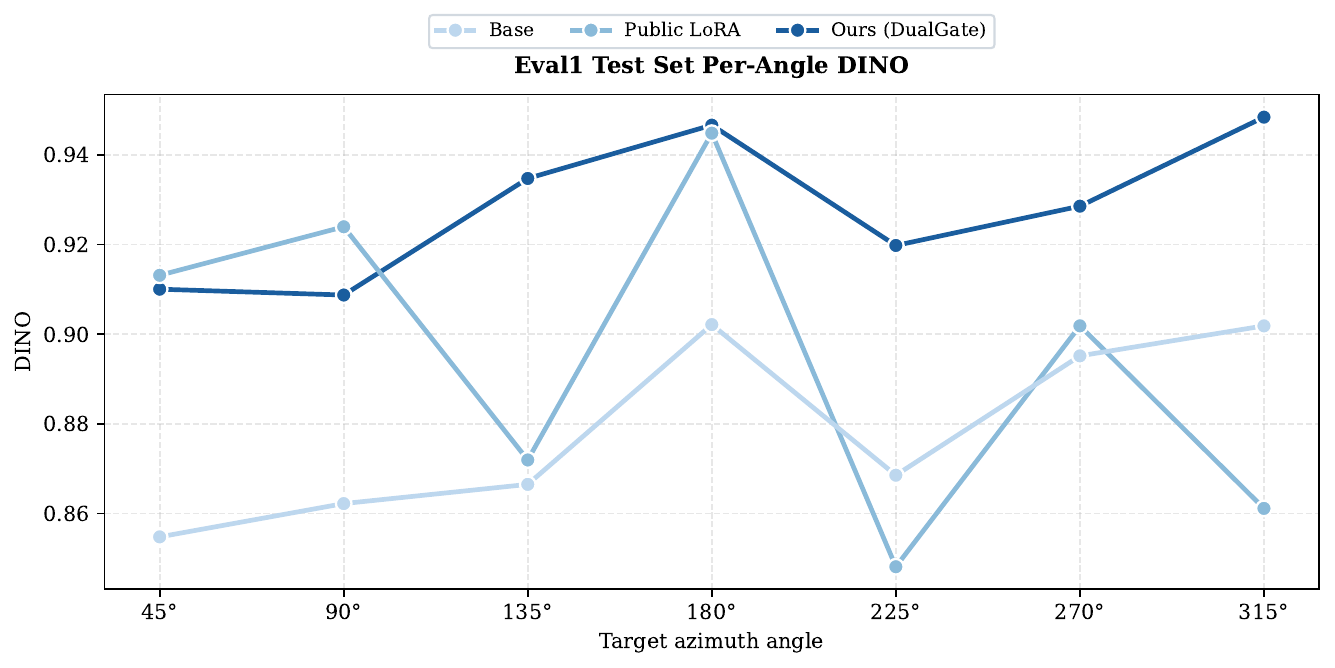}
\caption{Per-angle DINO audit for the Eval1 Test Set. The identity-consistency advantage of Ours persists at the angle level.}
\label{fig:v4-testset-per-angle-dino}
\end{figure}
