# Supplementary material for: DataEvolver: Let Your Data Build and Improve Itself via Goal-Driven Loop Agents
Source: arXiv:2605.01789 source file (2026-05-03)
Supplement: Supplementary file 2 [file r3_supplemented_angles_booktabs.tex]

% Auto-generated by scripts/generate_feedback_ablation_assets.py
\begin{tabular}{rrrrrrrrrr}
\toprule
Angle & PSNR exp5 & PSNR R1 & PSNR R3 & $\Delta$ & View exp5 & View R1 & View R3 & $\Delta$ & Verdict \\
\midrule
135 & 16.08 & 16.12 & 16.33 & +0.25 & 0.5574 & 0.6066 & 0.5738 & +0.0164 & gain \\
225 & 15.73 & 15.78 & 15.76 & +0.03 & 0.7541 & 0.7541 & 0.7541 & +0.0000 & gain \\
270 & 16.64 & 16.62 & 16.65 & +0.01 & 0.9016 & 0.8852 & 0.8689 & -0.0327 & mixed \\
315 & 16.33 & 16.26 & 16.35 & +0.02 & 0.5902 & 0.6230 & 0.7213 & +0.1311 & gain \\
\bottomrule
\end{tabular}
